# Supplementary material for: Decision-oriented benchmarking to transform AI weather forecast access: Application to the Indian monsoon
Source: arXiv:2602.03767 ancillary file (2026-02-03)
Supplement: Supplementary file 1 [file SI_monsoon_onset_benchmarking.pdf]

Supplementary Information for:

# Decision-oriented benchmarking to transform AI weather forecast access: Application to the Indian monsoon

Rajat Masiwal[1], Colin Aitken[2,†], Adam Marchakitus[1,†], Mayank Gupta[3], Katherine Kowal[4], Hamid Pahlavan[4,5], Tyler Yang[6], Y. Qiang Sun[1], Michael Kremer[2,7,8], Amir Jina[8,*], William R. Boos[6,9,*], Pedram Hassanzadeh[1,4,*]

[1]Department of the Geophysical Sciences, University of Chicago, IL, 60637
[2]Development Innovation Lab, University of Chicago, IL, 60637
[3]Development Innovation Lab India, University of Chicago Trust, India, 560025
[4]Data Science Institute, University of Chicago, IL, 60637
[5]NorthWest Research Associates, Boulder, CO, 80301
[6]Department of Earth and Planetary Science, University of California, Berkeley, Berkeley, California, 94720
[7]Kenneth C. Griffin Department of Economics, University of Chicago, IL, 60637
[8]Harris School of Public Policy, University of Chicago, IL, 60637
[9]Climate and Ecosystem Sciences Division, Lawrence Berkeley National Laboratory, Berkeley, California, 94720
[*]Corresponding authors: amirjina@uchicago.edu, william.boos@berkeley.edu, pedramh@uchicago.edu
[†]Equal contributions

- Supplementary Table S1 to S6
- Supplementary Figure S1 to S11

| Model | 1–15 Day | | | 16–30 Day | | |
|---|---|---|---|---|---|---|
| | MAE | FAR | MR | MAE | FAR | MR |
| Climatology | 5.7±0.5 **(7.2±1)** | 17% | **42%** | 6.9±0.8 (7.2±1) | **30%** | 23% |
| IFS* | 3.8±0.4 | 17% | 19% (10%) | 6.7±0.4 | 31% | 16% (0%) |
| AIFS† | 3.9±0.3 | 20% | 18% (12%) | 7.4±0.6 | 37% | 17% (3%) |
| FuXi | **3.1±0.3** | **7%** | 41% (20%) | 7.6±0.5 | 34% | **29%** (7%) |
| GraphCast | 4.5±0.4 | **24%** | **15%** (10%) | **8.9±0.4** | **48%** | **10%** (2%) |
| GenCast | 3.1±0.4 | 11% | 30% (15%) | **6.2±0.3** | 31% | 23%(7%) |
| FuXi-S2S* | 3.8±0.3 | 14% | 30% (23%) | 7.3±0.5 | 35% | 19% (10%) |
| NGCM | 3.4±0.4 | 16% | 25% (10%) | 7.1±0.4 | 38% | 14% (2%) |

**Supplementary Table S1:** Deterministic skill of models in forecasting monsoon onset in CMZ for the recent test period (2019–2024). Metrics shown are MAE (in days), FAR, and MR. For climatology, values in parentheses denote MAE when a fixed climatological onset date is used as the predictor; for MR, they indicate the percentage of complete misses (see Methods). The symbol † denotes forecast periods that include model training or finetuning years. An asterisk (*) indicates some years unavailable for that model in this period. Bold black values within each column indicate the lowest values (best skill), while bold red values indicate the highest values (worst skill). In columns where climatology exhibits the worst skill, the worst-performing AI model is also highlighted in red.

| No. | Label | Years included | Remarks |
|---|---|---|---|
| 1 | Recent test period | 2019–2024 | Modern testing period which includes some finetuning years for AIFS. For IFS and FuXi-S2S, data are available until 2023 and 2021, respectively. |
| 2 | Extended period | 1965–1978 and 2019–2024 | Longer testing period with 20 years of testing data for AIFS, FuXi, GraphCast and NGCM. |
| 3 | All available years | 1965–2024 | All the available years for each model (see Extended Data Table 1) |
| 4 | Common period | 2004–2021 | Period with a common set of 18 years for all models except for GenCast due to its high computational cost. |

**Supplementary Table S2:** Different periods analyzed in this study.

| Model | 1–15 Day | | | 16–30 Day | | |
|---|---|---|---|---|---|---|
| | **MAE** | **FAR** | **MR** | **MAE** | **FAR** | **MR** |
| Climatology | **6.6±0.6** (**8±0.6**) | 17% | **48%** | 7.8±0.7 (8±0.6) | 34% | **26%** |
| IFS* | 3.8±0.4 | 17% | 19% (10%) | 6.7±0.4 | 31% | 16% (0%) |
| AIFS† | 4.7±0.4 | 21% | 19% (8%) | 7.7±0.4 | 34% | 17% (2%) |
| FuXi | **3.4±0.2** | **10%** | 39% (20%) | 7.9±0.5 | 36% | 24% (6%) |
| GraphCast | 5.3±0.4 | **28%** | **13%** (6%) | **9.8±0.7** | **46%** | **9%** (2%) |
| GenCast | 3.7±0.3 | 15% | 26% (10%) | **6.6±0.5** | **33%** | 18% (3%) |
| FuXi-S2S†* | 3.7±0.3 | 14% | 30% (23%) | 7.3±0.5 | 35% | 19% (10%) |
| NGCM | 4.1±0.3 | 20% | 19% (6.5%) | 7.5±0.6 | 35% | 13% (1.5%) |

**Supplementary Table S3:** Same as Supplementary Table S1 but for the extended period (1965-1978 + 2019–2024).

| Model | 1–15 Day | | | 16–30 Day | | |
|---|---|---|---|---|---|---|
| | **MAE** | **FAR** | **MR** | **MAE** | **FAR** | **MR** |
| Climatology | **8.3±0.9** (**9.1±0.9**) | 20% | **52%** | 9±0.9 (9.1±0.9) | 36% | **30%** |
| IFS | 4.6±0.5 | 21% | 15% (4%) | 8±0.9 | 33% | 11% (0%) |
| AIFS† | 4.7±0.5 | 22% | 15% (7%) | 8.7±0.9 | 40% | 14% (2%) |
| FuXi† | 4±0.4 | **12%** | 35% (19%) | 8.4±0.5 | 37% | 23% (5%) |
| GraphCast† | 5.4±0.5 | **28%** | **7%** (5%) | **9.8±0.8** | **44%** | **8%** (1%) |
| FuXi-S2S† | **3.7±0.4** | 15% | 20% (12%) | **7.2±0.9** | **36%** | 11% (5%) |
| NGCM† | 4.5±0.5 | 22% | 15% (5%) | 7.9±0.8 | 38% | 10% (0.6%) |

**Supplementary Table S4:** Same as Supplementary Table S1 but for the common period (2004–2021). Note that due to the high computational cost of GenCast, hindcasts were not produced for 2004-2018.

| Model | 1–15 Day | | | 16–30 Day | | |
|---|---|---|---|---|---|---|
| | MAE | FAR | MR | MAE | FAR | MR |
| Climatology | **7.1±0.4 (8.2±0.4)** | 18% | **49%** | 8.1±0.4 (8.2±0.4) | 34% | **27%** |
| IFS* | 4.4±0.4 | 21% | 16% (4%) | 7.8±0.8 | 33% | 11% (0%) |
| AIFS† | 4.4±0.2 | 20% | 18% (7%) | 7.8±0.4 | 35% | 16% (2%) |
| FuXi† | **3.4±0.2** | **10%** | 40% (22%) | 7.8±0.3 | **33%** | 25% (7%) |
| GraphCast† | 5.2±0.2 | **28%** | **9%** (4%) | **9.2±0.4** | **42%** | **8%** (1%) |
| GenCast†* | 3.7±0.3 | 15% | 26% (10%) | **6.6±0.5** | 33% | 18% (3%) |
| FuXi-S2S†* | 3.6±0.4 | 15% | 20% (12%) | 7±0.8 | 35% | 12% (5%) |
| NGCM† | 4±0.2 | 19% | 18% (6%) | 7.1±0.4 | 34% | 11% (0.5%) |

**Supplementary Table S5:** Same as Supplementary Table S1 but for all available years in 1965–2024.

| Forecast Type | Metric | Climatology | AIFS | NGCM |
|---|---|---|---|---|
| Deterministic (1–15 day) | MAE(days) | 6 | 1.9 | 3.2 |
| | FAR(%) | 17.5 | 6.5 | 11.7 |
| | MR(%) | 39 | 4.5 | 27 |
| Deterministic (16–30 day) | MAE(days) | 6 | 6 | 5.5 |
| | FAR(%) | 28.6 | 29.1 | 38.5 |
| | MR(%) | 17.6 | 17.6 | 10.6 |
| Probabilistic (1–15 day) | AUC | 0.94 | - | 0.95 |
| | BSS(%) | 0 | - | 4 |
| | RPSS(%) | 0 | - | -1.3 |
| Probabilistic (1–30 day) | AUC | 0.898 | - | 0.87 |
| | BSS(%) | 0 | - | -3.6 |
| | RPSS(%) | 0 | - | -15.8 |

**Supplementary Table S6:** Same as Extended Data Table 2 but for AIWP models initialized with operational analysis data (see Extended Data Figure 5).

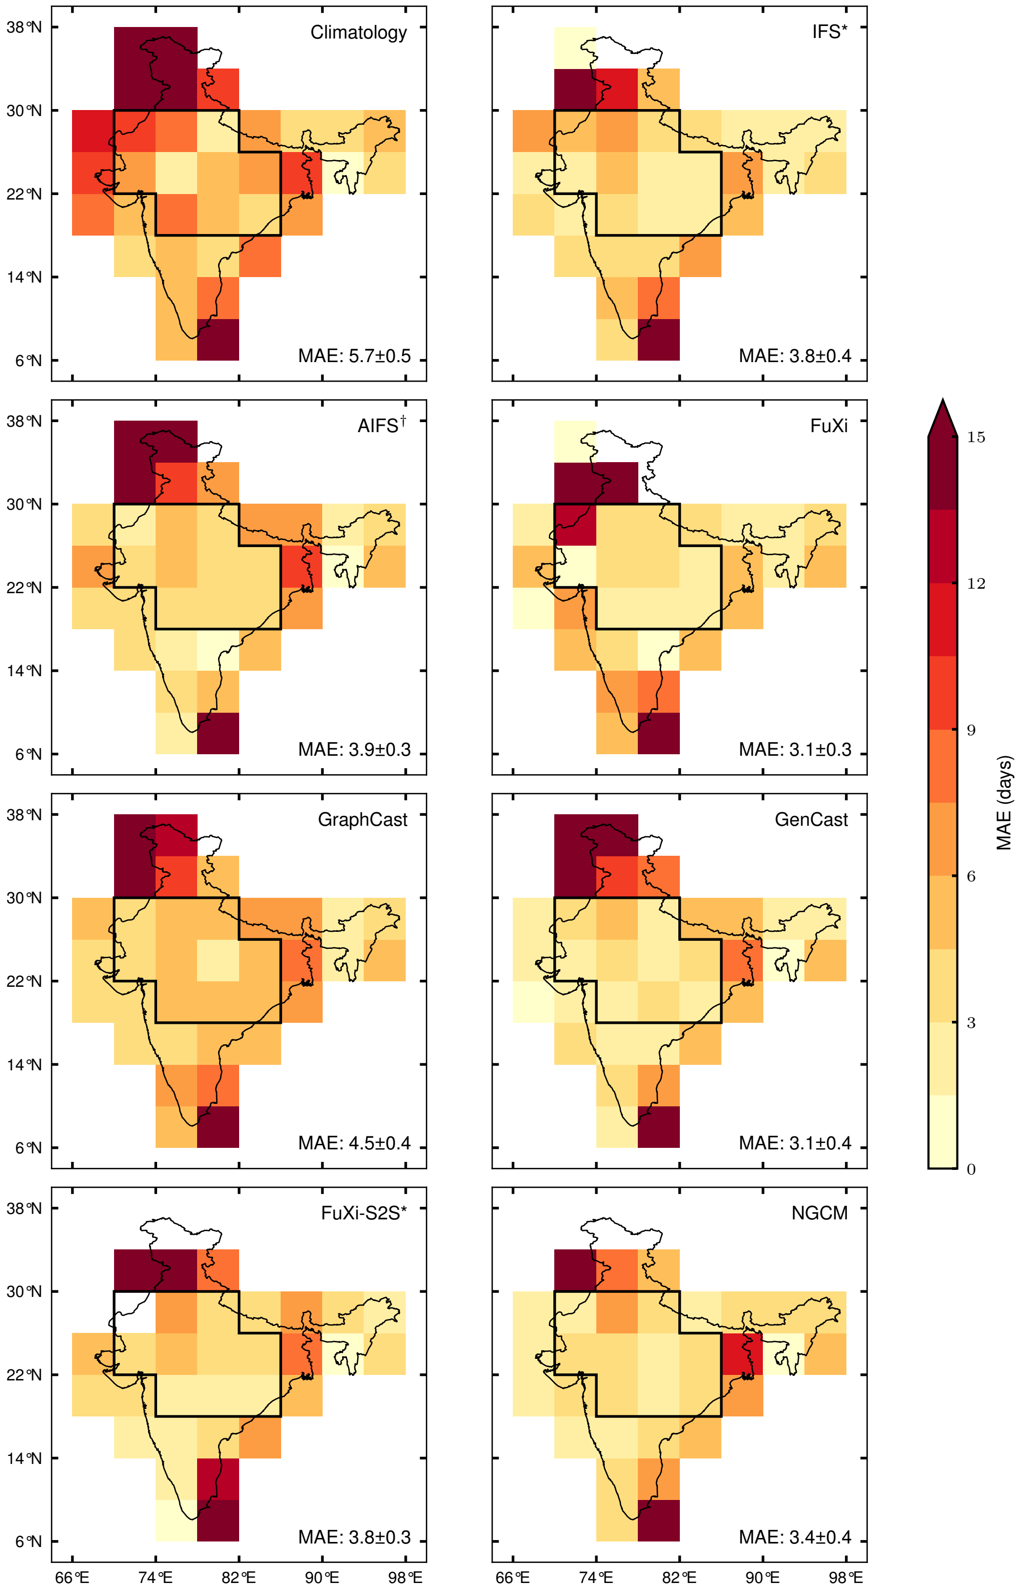


**Supplementary Figure S1:** Mean absolute error (MAE, in days) of all the models benchmarked in this study for 1-15 day forecasts during the 2019-2024 period. The number in each panel indicates the averaged MAE for CMZ (outlined in black).

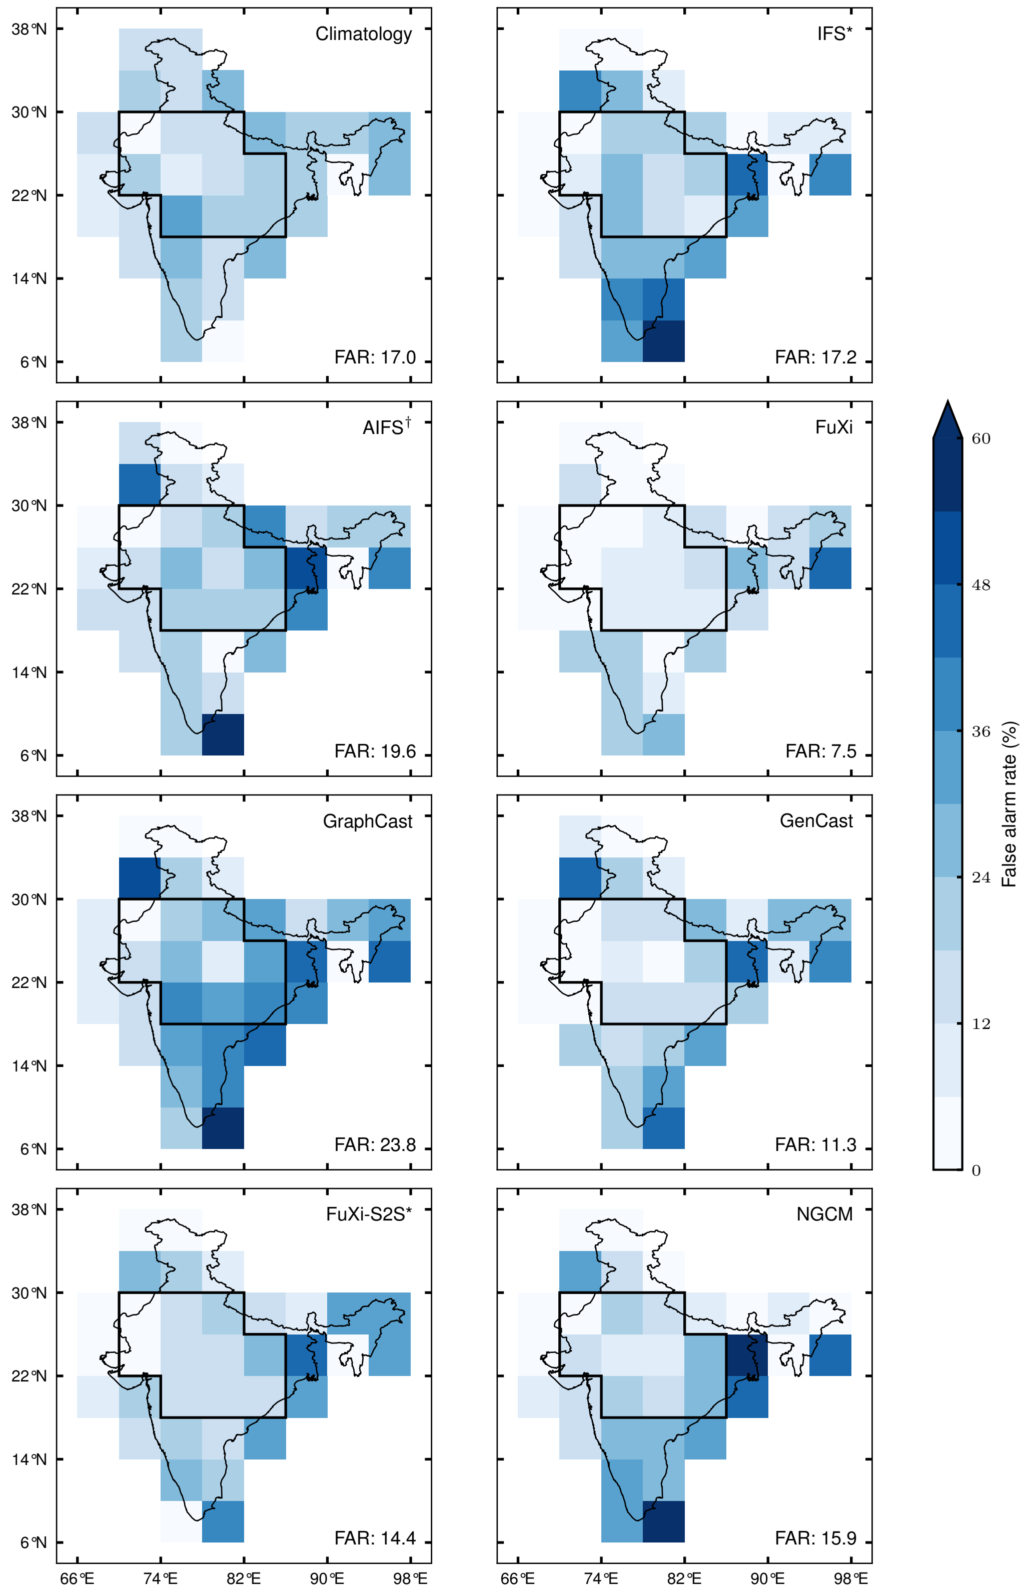


**Supplementary Figure S2:** False alarm rate (FAR, in %) of all the models benchmarked in this study for 1-15 day forecasts during the 2019-2024 period. The number in each panel indicates the averaged FAR for CMZ (outlined in black).

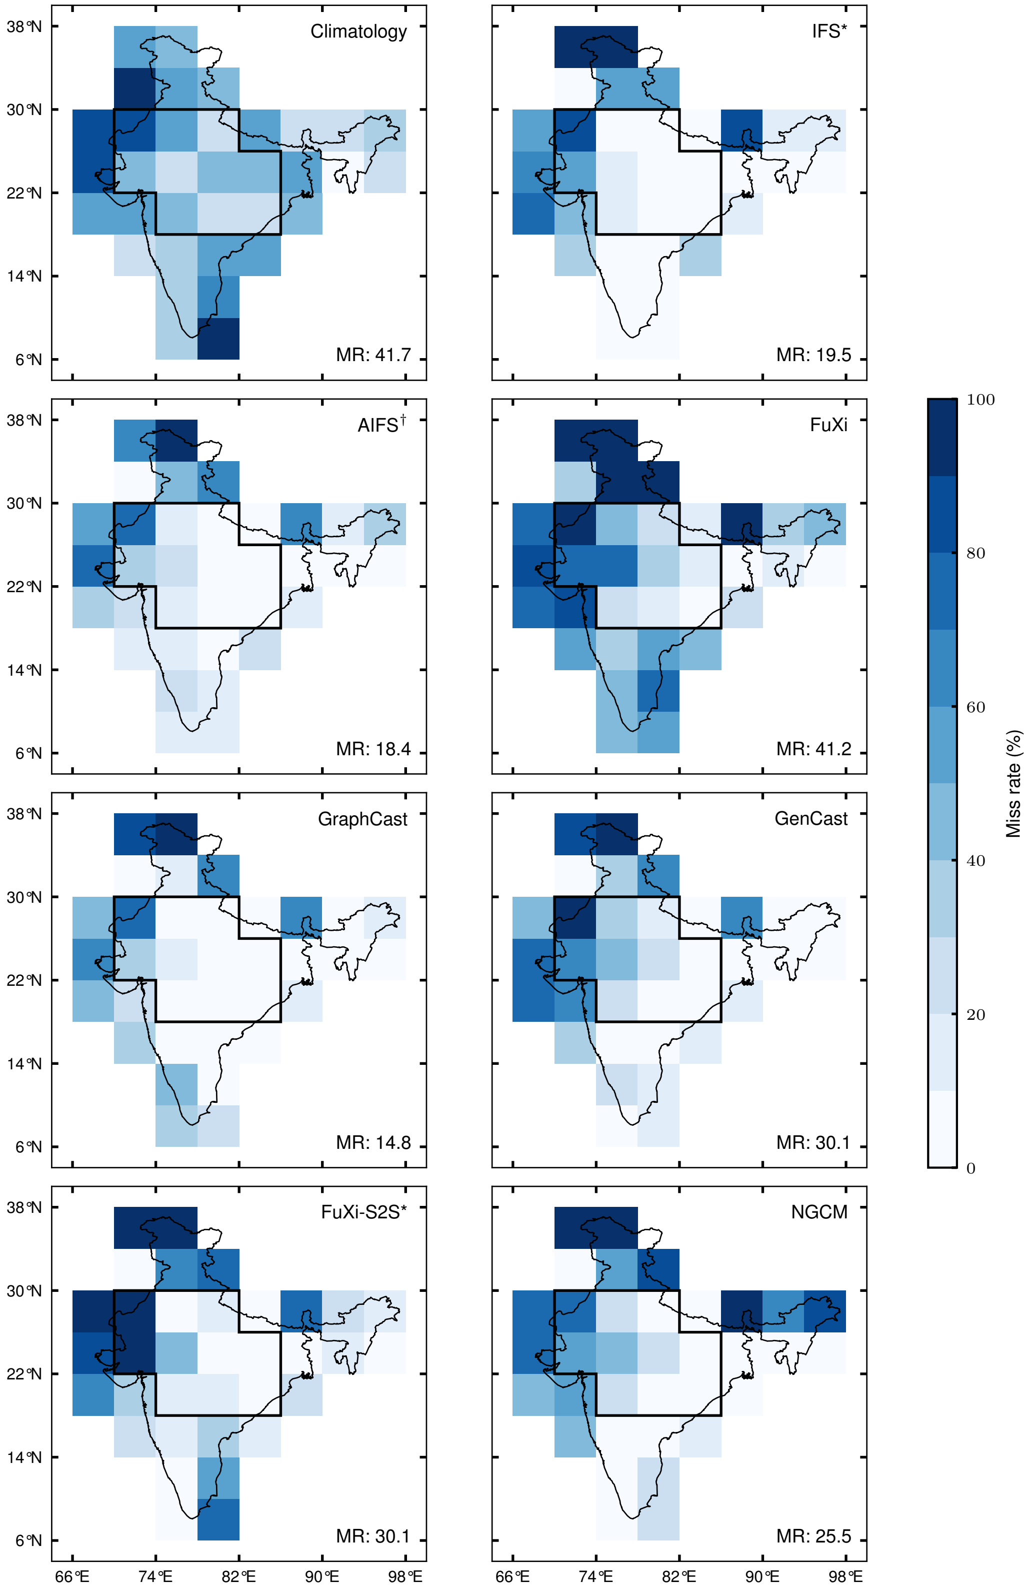


**Supplementary Figure S3:** Miss rate (MR, in %) of all the models benchmarked in this study for 1-15 day forecasts during the 2019-2024 period. The number in each panel indicates the averaged MR for the CMZ (outlined in black).

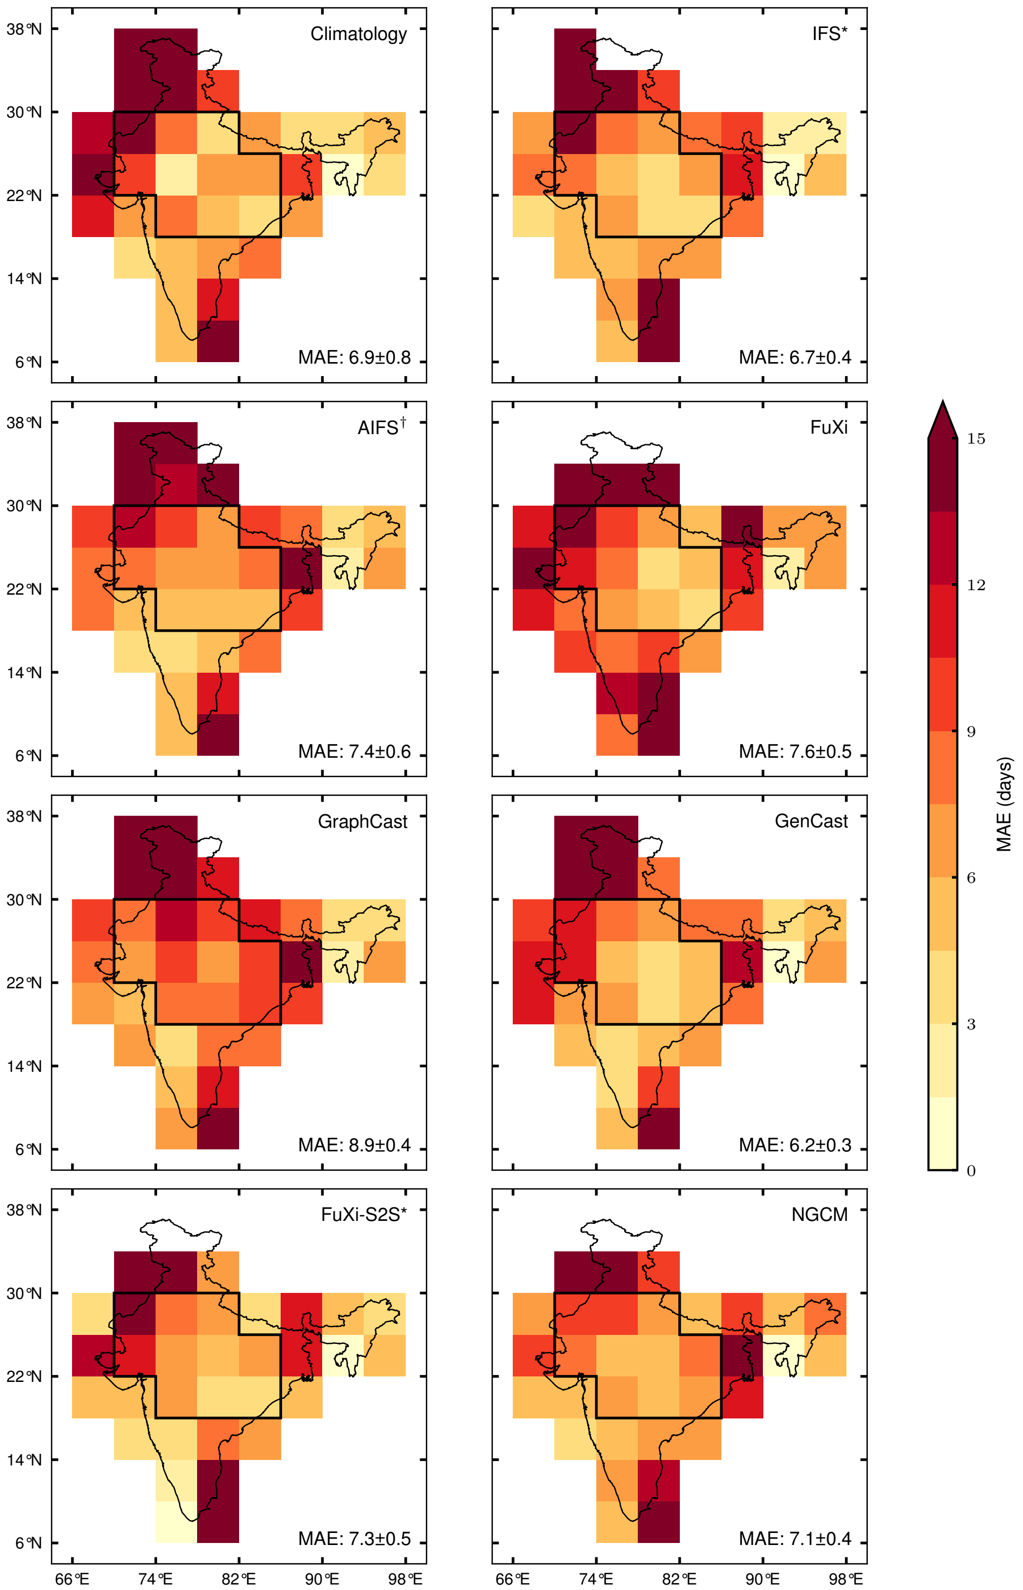


**Supplementary Figure S4:** Mean absolute error (MAE, in days) of all the models benchmarked in this study for 16-30 day forecasts during the 2019-2024 period. The number in each panel indicates the averaged MAE for CMZ (outlined in black).

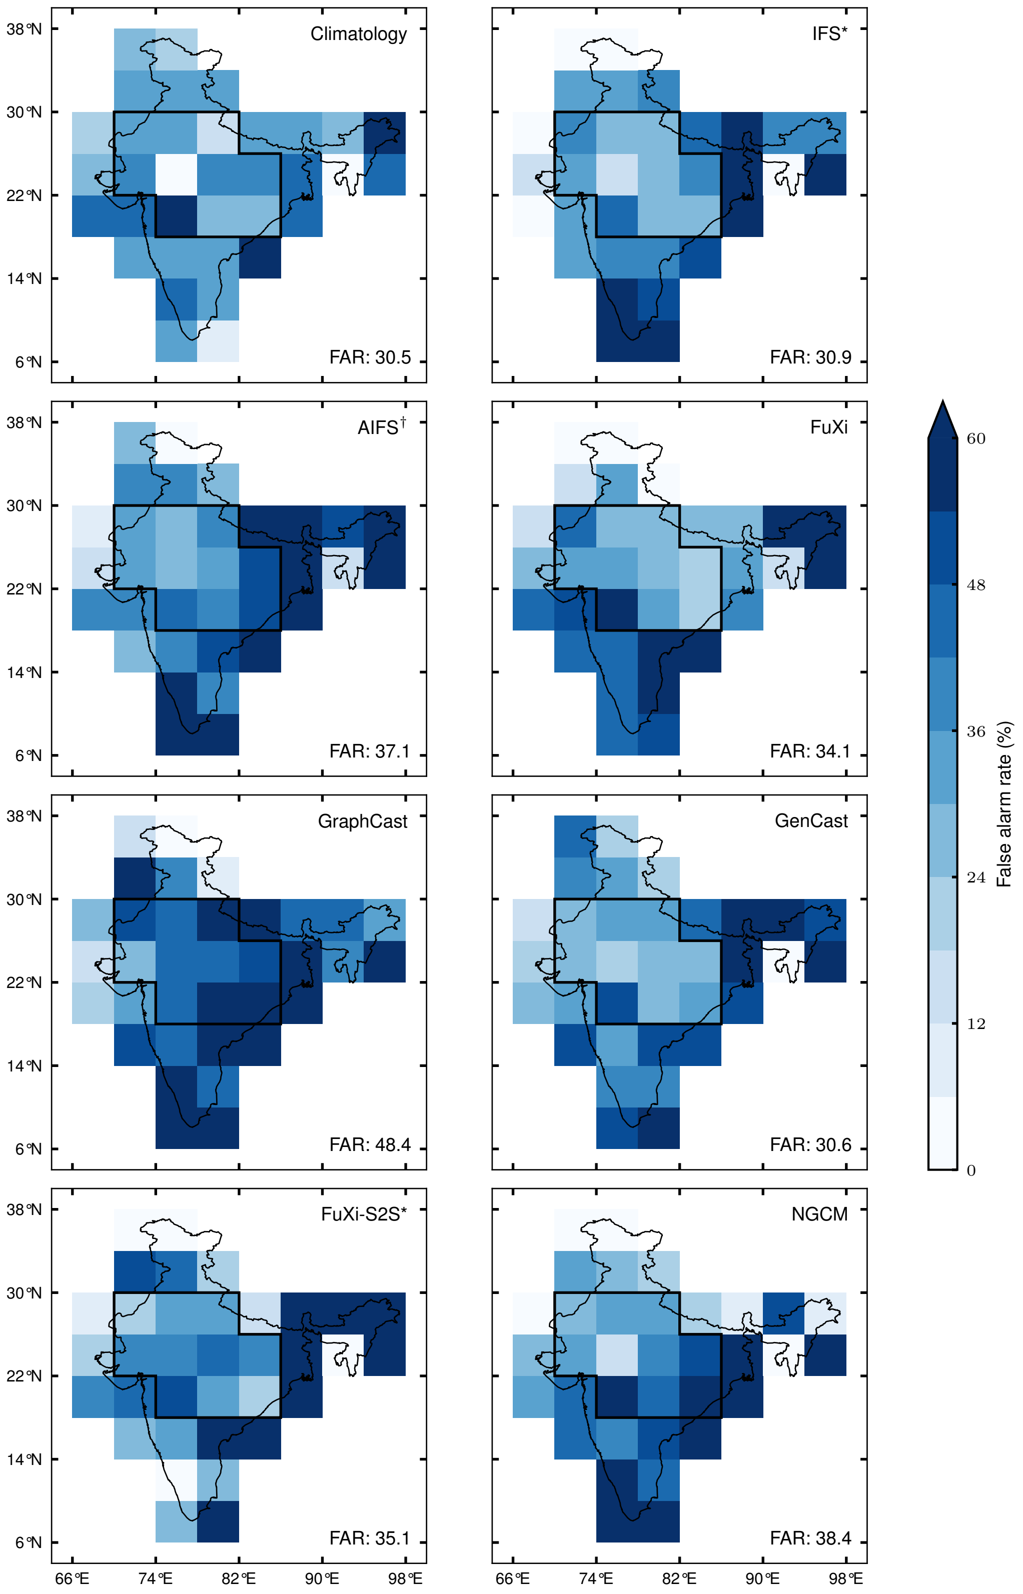


**Supplementary Figure S5:** False alarm rate (FAR, in %) of all the models benchmarked in this study for 16-30 day forecasts during the 2019-2024 the period. The number in each panel indicates the averaged FAR for CMZ (outlined in black).

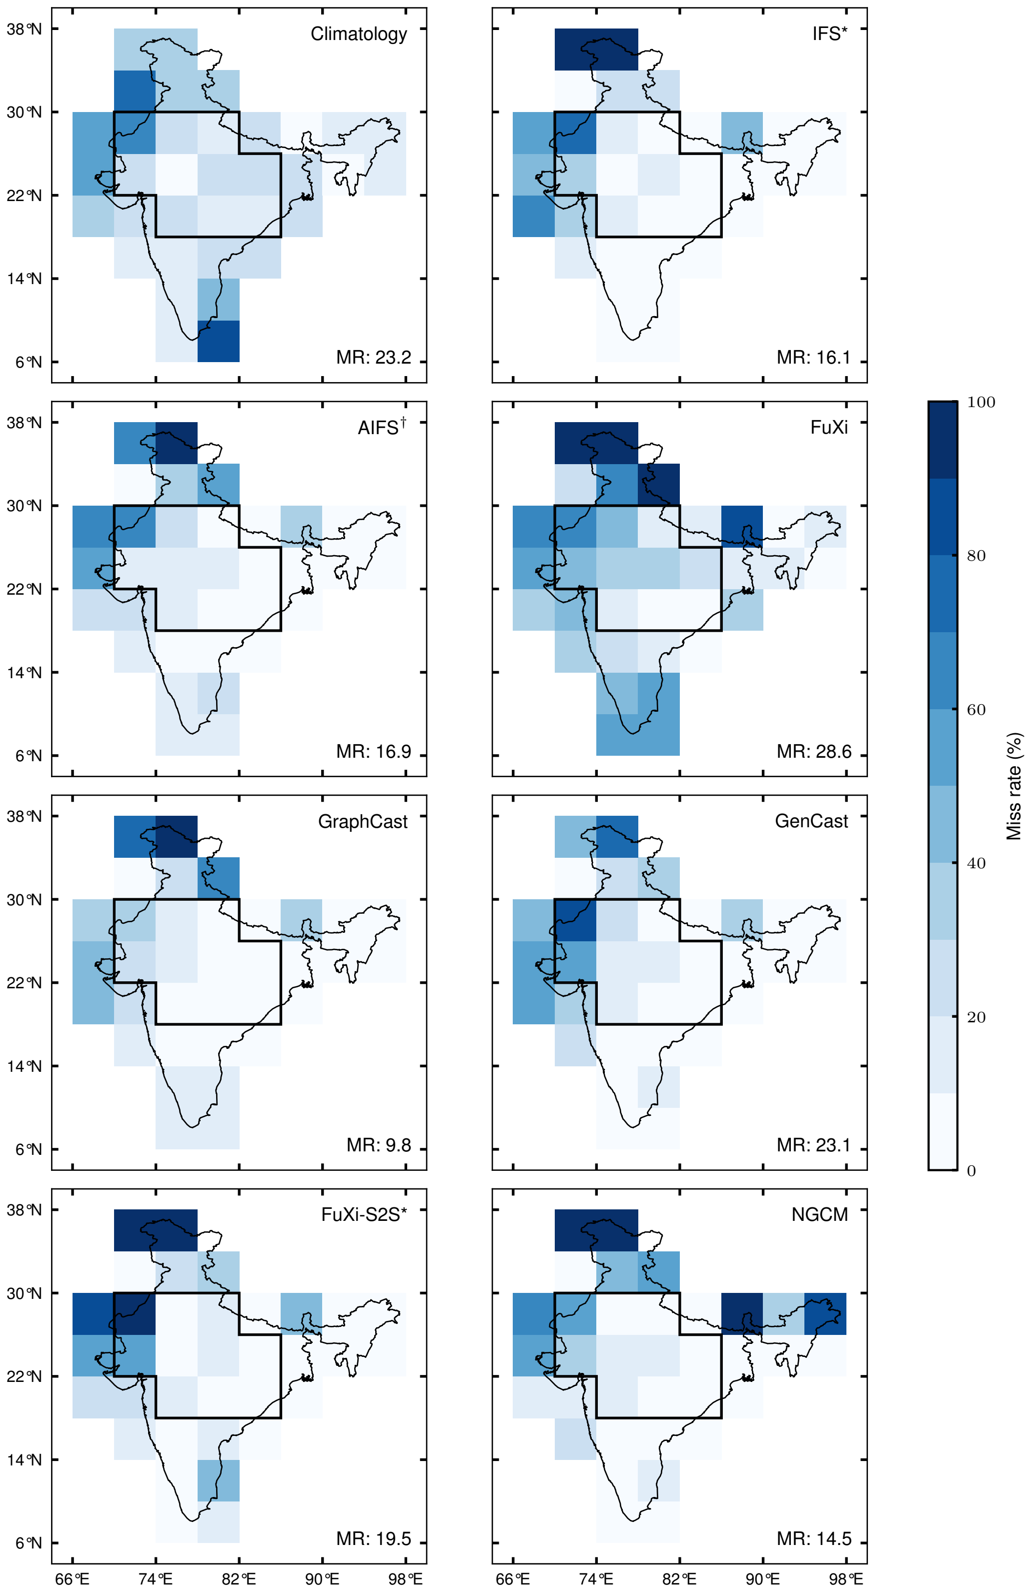


**Supplementary Figure S6:** Miss rate (MR, in %) of all the models benchmarked in this study for 16-30 day forecasts during the 2019-2024 period. The number in each panel indicates the averaged MR for CMZ (outlined in black).

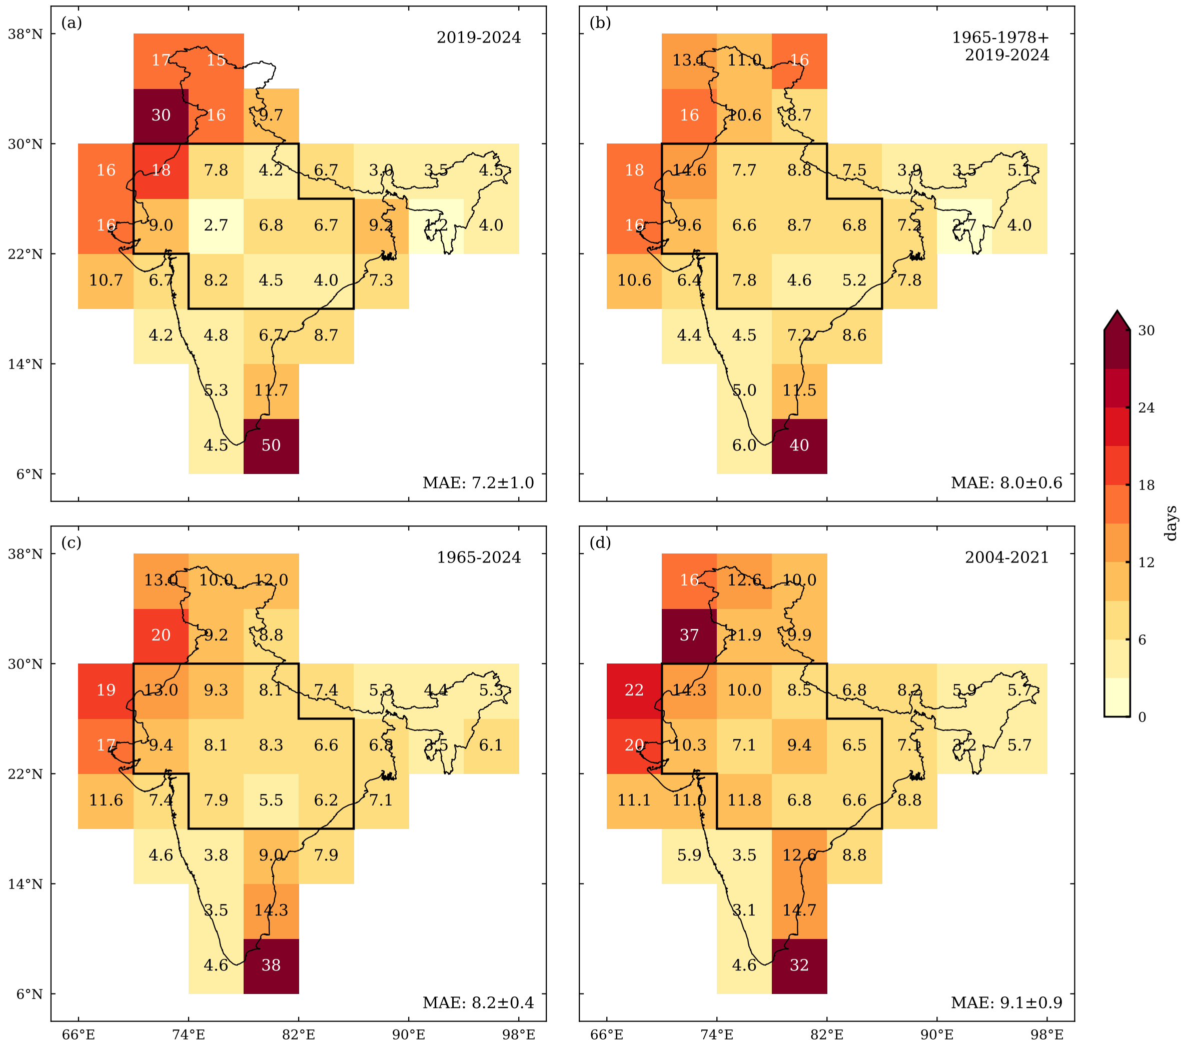


**Supplementary Figure S7:** Mean absolute error (MAE, in days) for a fixed climatological forecast (see Methods) for different periods labeled on each panel. The area averaged value for CMZ (outlined in black) is also indicated in each panel.

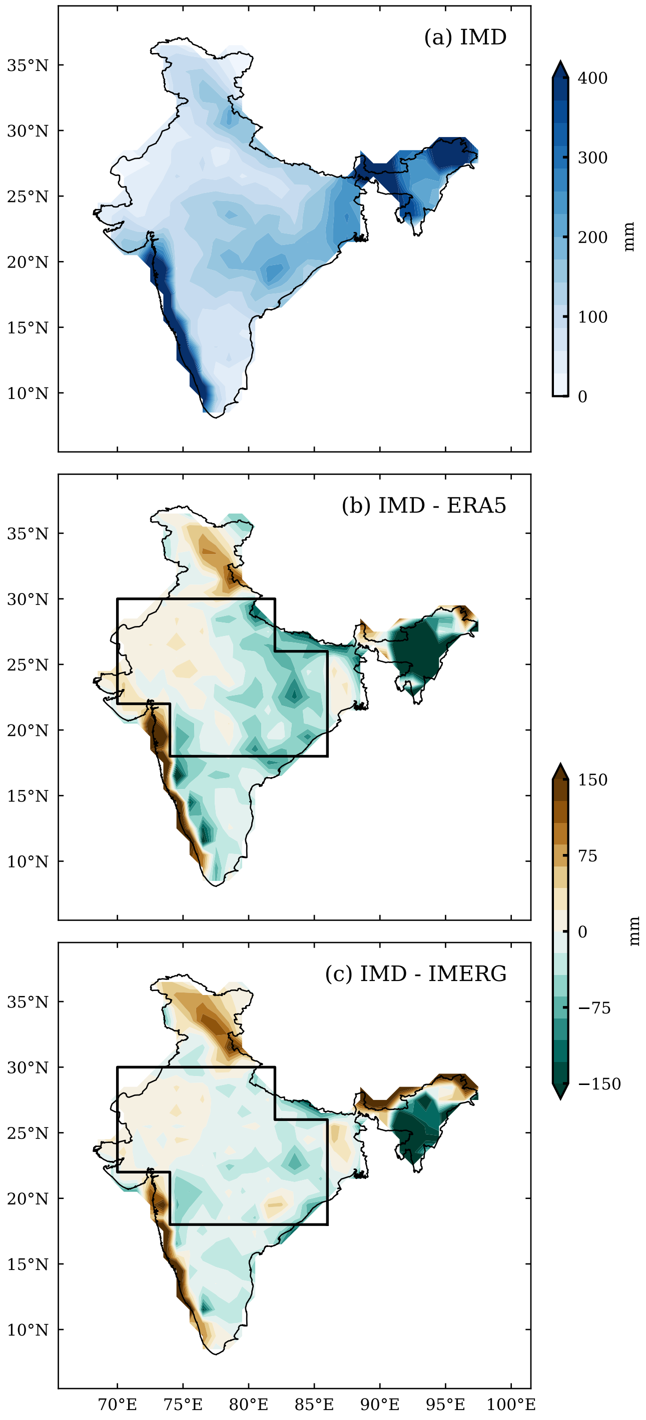


**Supplementary Figure S8:** (a) IMD 1° accumulated June rainfall averaged for the period 2002-2018. (b)-(c) Mean bias in ERA5 and IMERG compared to IMD 1° gridded rainfall for the same period. The CMZ is outlined in black.

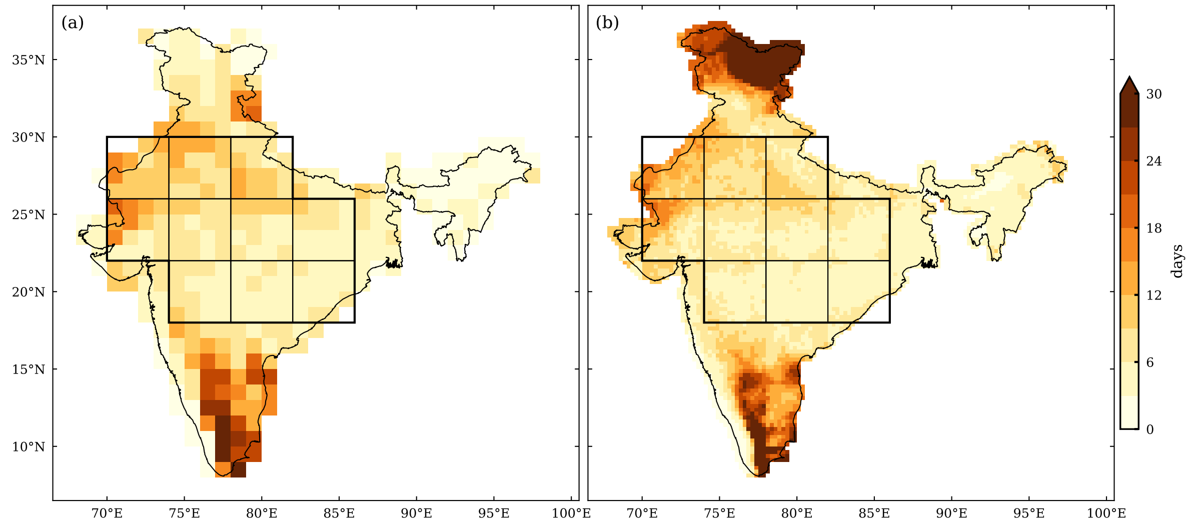


**Supplementary Figure S9:** (a) Mean subgrid variability of onset dates computed as the mean absolute difference in onset date within each 1° grid contained in the larger 4° grid in the IMD rain-gauge data for the period of 1901-2024. (b) Same as (a) but for IMD's 0.25° data. Note that for (b), the 4° grid onset dates are still obtained from regridding the 1° IMD data. Note that the IMD 0.25° gridded dataset is constructed from a varying number of rain-gauge observations over the analysis period.

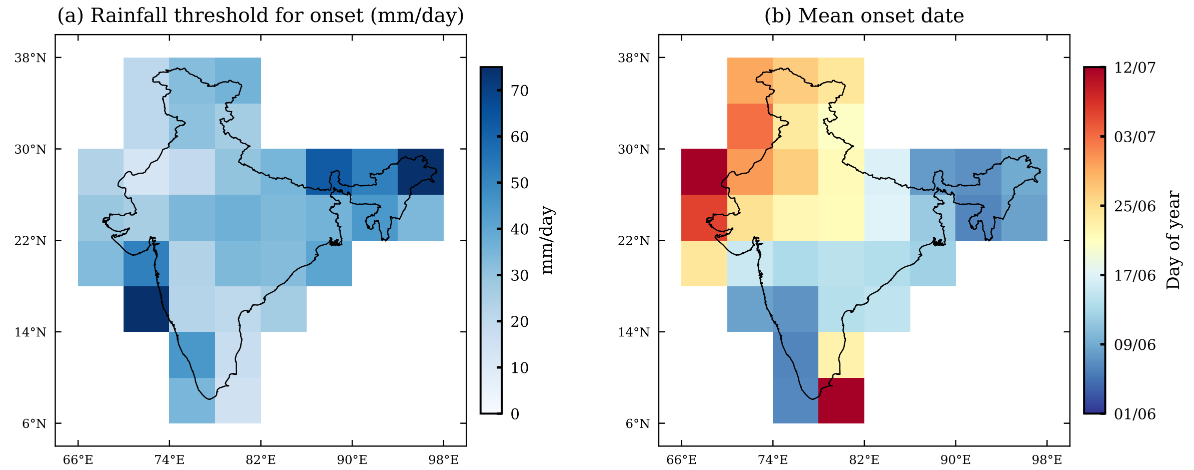


**Supplementary Figure S10:** (a) Climatological five-day accumulated rain threshold (in mm/day) for the first wet spell based on IMD rainfall data for 1901-2024. (b) Climatological onset date (with MOK filter) for the same time period. The north-westward progression of onset dates over the CMZ is observed in (b).

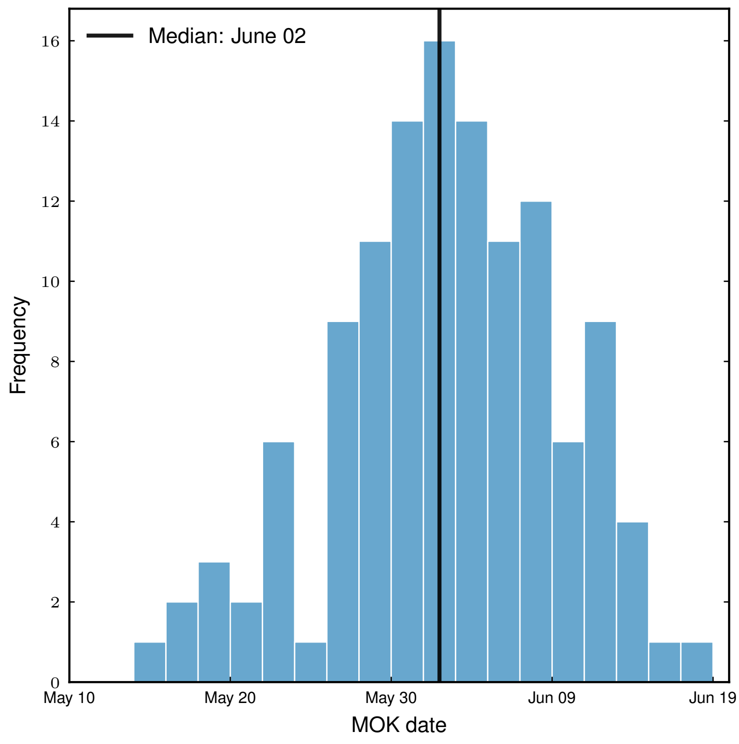


**Supplementary Figure S11:** Distribution of dates for monsoon onset over Kerala (MOK) for the period of 1901-2024. The median date from this distribution (June 2) is used to define the monsoon onset, which is the first wet spell that occurs after the median climatological MOK date.
